# Supplementary material for: Probing weak dipole-dipole interaction using phase-modulated non-linear spectroscopy
Source: arXiv:1702.07785 source file (2017-05-26)
Supplement: Supplementary file 1 [file SuppInfo.pdf]

# Supporting Information for "Probing weak dipole-dipole interaction using phase-modulated wave packet interferometry"

Zeng-Zhao Li,[†] Lukas Bruder,[§] Frank Stienkemeier,[§] and Alexander Eisfeld[†]
[†] *Max Planck Institute for the Physics of Complex Systems, Nöthnitzer Strasse 38, 01187 Dresden, Germany and*
[§] *Physikalisches Institut, Universität Freiburg, Hermann-Herder-Strasse 3, 79104 Freiburg, Germany*

In this Supporting Information we provide details on our numerical implementation and details of the perturbation theory used in the main paper.

## I. DETAILS ON THE NUMERICAL IMPLEMENTATION

### A. Effective Hamiltonian in the rotating frame

To speed up the numerical simulations we perform a rotating wave approximation. The following derivation of the corresponding equation of motion is done for identical carrier frequencies of the two pulses, i.e. $\omega_1 = \omega_2 = \omega_{\rm L}$.

Our aim is to solve the time-dependent Schrödinger equation $\partial_t|\Psi(t)\rangle = -iH(t)|\Psi(t)\rangle$ with $H(t)$ given by Eq. (1) of the main text. To this end we transform to a rotating frame via the transformation $|\tilde{\Psi}(t)\rangle = e^{iSt}|\Psi(t)\rangle$. We work in the eigenstate representation of the dipole-dipole interacting particles, which is given in Fig. 2 of the main text. Then the matrix $S$ is given by

$$\begin{aligned} S \;=\; & (\omega_{\rm L}+2\epsilon_{\rm g})\Big(|\psi^+_{\rm ge}\rangle\langle\psi^+_{\rm ge}| + |\psi^-_{\rm ge}\rangle\langle\psi^-_{\rm ge}| + |\psi^+_{\rm gf}\rangle\langle\psi^+_{\rm gf}| + |\psi^-_{\rm gf}\rangle\langle\psi^-_{\rm gf}|\Big) \\ & +2(\omega_{\rm L}+\epsilon_{\rm g})\Big(|\psi_{\rm ee}\rangle\langle\psi_{\rm ee}| + |\psi^+_{\rm ef}\rangle\langle\psi^+_{\rm ef}| + |\psi^-_{\rm ef}\rangle\langle\psi^-_{\rm ef}| + |\psi_{\rm ff}\rangle\langle\psi_{\rm ff}|\Big). \end{aligned} \tag{S1}$$

The first row contains terms with one excitation, the second row terms with two excitations. Finally, after dropping counter-rotating terms we arrive at the equation

$$\partial_t|\tilde{\Psi}(t)\rangle = -i\tilde{H}(t)|\tilde{\Psi}(t)\rangle \tag{S2}$$

with

$$\begin{aligned} \tilde{H} \;=\; & \tilde{\omega}^+_{\rm ge}|\psi^+_{\rm ge}\rangle\langle\psi^+_{\rm ge}| + \tilde{\omega}^-_{\rm ge}|\psi^-_{\rm ge}\rangle\langle\psi^-_{\rm ge}| + \tilde{\omega}^+_{\rm gf}|\psi^+_{\rm gf}\rangle\langle\psi^+_{\rm gf}| + \tilde{\omega}^-_{\rm gf}|\psi^-_{\rm gf}\rangle\langle\psi^-_{\rm gf}| \\ & +\tilde{\omega}_{\rm ee}|\psi_{\rm ee}\rangle\langle\psi_{\rm ee}| + \tilde{\omega}_{\rm ff}|\psi_{\rm ff}\rangle\langle\psi_{\rm ff}| + \tilde{\omega}^+_{\rm ef}|\psi^+_{\rm ef}\rangle\langle\psi^+_{\rm ef}| + \tilde{\omega}^-_{\rm ef}|\psi^-_{\rm ef}\rangle\langle\psi^-_{\rm ef}| \\ & -\sqrt{2}\mu_{\rm e}\tilde{E}(t)\big(|\psi_{\rm gg}\rangle\langle\psi^+_{\rm ge}| + |\psi^+_{\rm ge}\rangle\langle\psi_{\rm ee}|\big) - \sqrt{2}\mu_{\rm f}\tilde{E}(t)\big(|\psi_{\rm gg}\rangle\langle\psi^+_{\rm gf}| + |\psi^+_{\rm gf}\rangle\langle\psi_{\rm ff}|\big) \\ & -\mu_{\rm e}\tilde{E}(t)\big(|\psi^+_{\rm gf}\rangle\langle\psi^+_{\rm ef}| + |\psi^-_{\rm gf}\rangle\langle\psi^-_{\rm ef}\big) - \mu_{\rm f}\tilde{E}(t)\big(|\psi^+_{\rm ge}\rangle\langle\psi^+_{\rm ef}| - |\psi^-_{\rm ge}\rangle\langle\psi^-_{\rm ef}\big) + H.c., \end{aligned} \tag{S3}$$

where $\tilde{\omega}_{\rm ee} = 2(\omega_{\rm eg}-\omega_{\rm L})$, $\tilde{\omega}_{\rm ff} = 2(\omega_{\rm fg}-\omega_{\rm L})$, $\tilde{\omega}^\pm_{\rm ge} = \omega_{\rm eg} \pm V_{\rm ee} - \omega_{\rm L}$, $\tilde{\omega}^\pm_{\rm gf} = \omega_{\rm fg} \pm V_{\rm ff} - \omega_{\rm L}$, $\tilde{\omega}^\pm_{\rm ef} = \omega_{\rm eg} + \omega_{\rm fg} - 2\omega_{\rm L}$ with $\omega_{\rm eg} = \epsilon_{\rm e} - \epsilon_{\rm g}$ and $\omega_{\rm fg} = \epsilon_{\rm f} - \epsilon_{\rm g}$, and

$$\tilde{E}(t) = \sum_{j=1}^{2} \frac{A_j(t-t_j-\tau_m)}{2} e^{-i[\omega_{\rm L}(t_j+\tau_m)-(\Omega_j\tau_m+\phi^0_j)]}. \tag{S4}$$

We numerically solve Eq. (S2) using the integrator 'lsoda' in Python.

### B. Numerically performing the demodulation

For an efficient numerical implementation of Eq. (9) of the main text we use that the fluorescence signal $S_{\rm Fluor}(t_{21},\tau_m)$ is a time-periodic function in $\tau_m$ with period $T = \frac{2\pi}{\Omega_{21}}$ with $\Omega_{21} = \Omega_2 - \Omega_1$ being the frequency difference between two acousto-optical modulators. One finds that

$$\tilde{S}_{\rm Fluor}(t_{21},\kappa) \;=\; \frac{1}{\tau_{\rm LI}(1-e^{-\frac{T}{\tau_{\rm LI}}})} \int_0^T d\tau_m S_{\rm Fluor}(t_{21},\tau_m)\, S_{\rm ref}(t_{21},\tau_m,\kappa) e^{-\frac{\tau_m}{\tau_{\rm LI}}}. \tag{S5}$$

To numerically calculate the integral, for given pulse delay $t_{21}$ and demodulation order $\kappa$, we use the sum of discrete values of the integrand at various $m$ (here $\tau_m = mT_{\rm Rep}$ and $m$ takes integer values) to represent the integral. In our simulation, we consider the demodulation up to the second order and then take 1000 as the maximal value of $m$ (with $T_{\rm Rep} = 1$ and $\tau_m \ll \tau_{\rm LI} = 10^8$) which is enough for the accuracy of our result.

The obtained signal from demodulation is further multiplied by a Gaussian window function $e^{-\frac{t_{21}^2}{2\sigma^2}}$ to avoid Fourier transform artefacts. The Fourier transformation of windowed signal gives the corresponding spectrum (such as the absorption and dispersion lineshapes). In our simulation, the *scipy.fftpack* package in python is used to implement the Fourier transformation. The number of sampling points used in the transformation, e.g., $y[k] = \sum_{n=0}^{N_{t_{21}}-1} e^{-2\pi i \frac{kn}{N_{t_{21}}}} x[n]$ is $N_{t_{21}} = 4500$. In order to increase the spectral resolution we add zeros to our data and also symmetrise the data points.

### C. Subtraction of pulse-overlap-induced broad backgrounds

In each second-harmonic spectrum presented in the main text, a broad background, caused by pulse overlap, has been subtracted. Exemplary spectra before and after subtracting this background are shown in Fig. S1(a) and (b), respectively. To achieve this subtraction, we use polynomial and Gaussian functions, $f_p(x) = a * \sum_{j=0}^{5} a_j * (x - x_0)^j$ and $f_g(y) = b * e^{-\frac{(y-y_0)^2}{2s^2}}$ to fit the broad backgrounds of the imaginary and real parts of a spectrum, respectively.

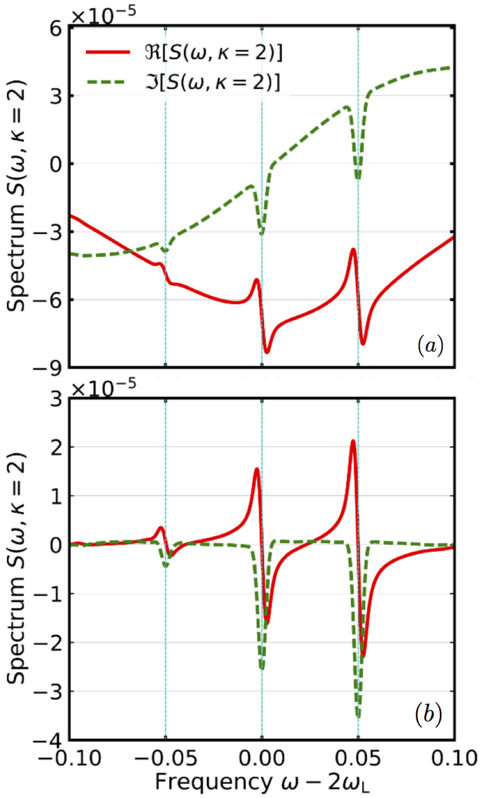


FIG. S1: (color online) The real (solid red line) and imaginary (dashed green line) parts of the 2HD spectrum $S(\omega, \kappa = 2)$ in Eq. (11) in the main text: (a) before and (b) after the subtraction of broad backgrounds. (b) is reproduced from Fig. 3(a2) in the main text.

## II. PERTURBATIVE TREATMENT

We work in the interaction picture defined by $|\Psi(t)\rangle_{\rm I} = e^{iH_0t}|\Psi(t)\rangle$ ($H_0 = H_1 + H_2 + V_{12}$ given by Eqs. (2) and (3) of the main text) that can be expanded as

$$|\Psi(t)\rangle_{\rm I} \; = \; \sum_n c_n(t)|n\rangle, \tag{S6}$$

where $|n\rangle \in \{|\psi_{\rm gg}\rangle, |\psi^+_{\rm ge}\rangle, |\psi^+_{\rm gf}\rangle, |\psi_{\rm ee}\rangle, |\psi^+_{\rm ef}\rangle, |\psi_{\rm ff}\rangle\}$ are the symmetric eigenstates of $H_0$. Note that antisymmetric basis states (i.e. $|\psi^-_{\rm ge}\rangle$, $|\psi^-_{\rm gf}\rangle$, and $|\psi^-_{\rm ef}\rangle$) don't enter the wave function because there are no corresponding pathways for particles excited from the initial state $|\psi_{\rm gg}\rangle$ (or equivalently the symmetric-state subspace is decoupled from the antisymmetric-state subspace). Insert the above expansion to the equation of motion $i\partial_t|\Psi(t)\rangle_{\rm I} = H_1^{\rm I}(t)|\Psi(t)\rangle_{\rm I}$ where $H_1^{\rm I}(t) = e^{iH_0t}H_1e^{-iH_0t}$ with $H_1 = H_1^{\rm int} + H_2^{\rm int}$ given by Eq. (5) of the main text, the time-dependent perturbation theory gives

$$c_n(t) \; = \; \delta_{ni} - i\int_{t_0}^{t} dt'\langle n|H_1^{\rm I}(t')|i\rangle - \int_{t_0}^{t} dt'\int_{t_0}^{t'} dt''\sum_m \langle n|H_1^{\rm I}(t')|m\rangle\langle m|H_1^{\rm I}(t'')|i\rangle + \cdots, \tag{S7}$$

where $i$ and $n$ denote the initial and final states respectively.

Inserting into the expression for $S_{\rm Fluor}(t_{21},\tau_m)$ (i.e. Eq. (7) in the main text) and keeping only terms containing up to four interactions we obtain

$$\begin{aligned} S_{\rm Fluor}(t_{21},\tau_m) \; &= \; \langle\Psi(T_{\rm F})|P_{\rm Fluor}|\Psi(T_{\rm F})\rangle = {}_I\langle\Psi(T_{\rm F})|e^{iH_0t}P_{\rm Fluor}e^{-iH_0t}|\Psi(T_{\rm F})\rangle_I = {}_I\langle\Psi(T_{\rm F})|P_{\rm Fluor}|\Psi(T_{\rm F})\rangle_I \\ &= \; p_{\psi^+_{\rm ge}} + p_{\psi^+_{\rm gf}} + 2(p_{\psi_{\rm ee}} + p_{\psi^+_{\rm ef}} + p_{\psi_{\rm ff}}), \end{aligned} \tag{S8}$$

with

$$p_{\psi^+_{\rm ge}} \; = \; |c_{\psi^+_{\rm ge}}|^2 = |c^{(1)}_{\psi^+_{\rm ge}}|^2 + \mathcal{A} + \mathcal{A}^*, \tag{S9}$$

$$p_{\psi^+_{\rm gf}} \; = \; |c_{\psi^+_{\rm gf}}|^2 = |c^{(1)}_{\psi^+_{\rm gf}}|^2 + \mathcal{B} + \mathcal{B}^*, \tag{S10}$$

$$p_{\psi_{\rm ee}} \; = \; |c_{\psi_{\rm ee}}|^2, \tag{S11}$$

$$p_{\psi_{\rm ff}} \; = \; |c_{\psi_{\rm ff}}|^2, \tag{S12}$$

$$p_{\psi^+_{\rm ef}} \; = \; |c_{\psi^+_{\rm ef}}|^2, \tag{S13}$$

where

$$\begin{aligned} \mathcal{A} \; &= \; (c^{(1)}_{\psi^+_{\rm ge}})^* c^{(3,1)}_{\psi^+_{\rm ge}} + (c^{(1)}_{\psi^+_{\rm ge}})^* c^{(3,\bar{1})}_{\psi^+_{\rm ge}} + (c^{(1)}_{\psi^+_{\rm ge}})^* c^{(3,2)}_{\psi^+_{\rm ge}} \\ &\quad + (c^{(1)}_{\psi^+_{\rm ge}})^* c^{(3,\bar{2})}_{\psi^+_{\rm ge}} + (c^{(1)}_{\psi^+_{\rm ge}})^* c^{(3,3)}_{\psi^+_{\rm ge}}, \end{aligned} \tag{S14}$$

$$\begin{aligned} \mathcal{B} \; &= \; (c^{(1)}_{\psi^+_{\rm gf}})^* c^{(3,1)}_{\psi^+_{\rm gf}} + (c^{(1)}_{\psi^+_{\rm gf}})^* c^{(3,\bar{1})}_{\psi^+_{\rm gf}} + (c^{(1)}_{\psi^+_{\rm gf}})^* c^{(3,2)}_{\psi^+_{\rm gf}} \\ &\quad + (c^{(1)}_{\psi^+_{\rm gf}})^* c^{(3,\bar{2})}_{\psi^+_{\rm gf}} + (c^{(1)}_{\psi^+_{\rm gf}})^* c^{(3,3)}_{\psi^+_{\rm gf}}. \end{aligned} \tag{S15}$$

The transition amplitudes with time-ordered triple integrals involved are shown below. In the derivation of these amplitudes, rapidly oscillating terms are dropped within the rotating-wave approximation. In addition, we use $(\omega_j - \Omega_j)(t' - t_j - \tau_m) \sim \omega_j(t' - t_j - \tau_m)$ because the laser frequency is much larger than the frequency of the acousto-optic modulator, i.e. $\omega_j(\sim THz) \gg \Omega_j(\sim kHz)$, and also $\Omega_j(t_j + \tau_m) \sim \Omega_j\tau_m$ because of longer repetition time than the pulse arrive time, i.e. $\tau_m(\sim ns) \gg t_j(\sim ps)$.

The transition amplitudes in Eqs. (S9)-(S13) are given as follows

$$c^{(1)}_{\psi^+_{\rm ge}}(t) \; = \; -\frac{i}{\sqrt{2}}\mu_{\rm e}\sum_{l=1}^{2}\int_0^t dt' A_j(t' - t_l - \tau_m)e^{i(\omega_{\rm eg}+V_{\rm ee}-\omega_j)(t'-t_j-\tau_m)}e^{i(\omega_{\rm eg}+V_{\rm ee})(t_l+\tau_m)-i(\Omega_j\tau_m+\phi_j^{(0)})}, \tag{S16}$$

$$c^{(3,1)}_{\psi^+_{\rm ge}}(t) = \frac{i}{4}\sqrt{2}\mu_{\rm e}^3 \sum_{l,n,s=1}^{2} \int_0^t dt' A_l(t'-t_l-\tau_m) e^{i(\omega_{\rm eg}+V_{\rm ee}-\omega_l)(t'-t_l-\tau_m)} e^{i(\omega_{\rm eg}+V_{\rm ee})(t_l+\tau_m)-i(\Omega_l\tau_m+\phi_l^{(0)})}$$
$$\times \int_0^{t'} dt'' A_n(t''-t_n-\tau_m) e^{-i(\omega_{\rm eg}+V_{\rm ee}-\omega_n)(t''-t_n-\tau_m)} e^{-i(\omega_{\rm eg}+V_{\rm ee})(t_n+\tau_m)+i(\Omega_n\tau_m+\phi_n^{(0)})}$$
$$\times \int_0^{t''} dt''' A_s(t'''-t_s-\tau_m) e^{i(\omega_{\rm eg}+V_{\rm ee}-\omega_s)(t'''-t_s-\tau_m)} e^{i(\omega_{\rm eg}+V_{\rm ee})(t_s+\tau_m)-i(\Omega_s\tau_m+\phi_s^{(0)})}, \quad \text{(S17)}$$

$$c^{(3,\bar{1})}_{\psi^+_{\rm ge}}(t) = \frac{i}{4}\sqrt{2}\mu_{\rm e}\mu_{\rm f}^2 \sum_{l,n,s=1}^{2} \int_0^t dt' A_l(t'-t_l-\tau_m) e^{i(\omega_{\rm eg}+V_{\rm ee}-\omega_l)(t'-t_l-\tau_m)} e^{i(\omega_{\rm eg}+V_{\rm ee})(t_l+\tau_m)-i(\Omega_l\tau_m+\phi_l^{(0)})}$$
$$\times \int_0^{t'} dt'' A_n(t''-t_n-\tau_m) e^{-i(\omega_{\rm fg}+V_{\rm ff}-\omega_n)(t''-t_n-\tau_m)} e^{-i(\omega_{\rm fg}+V_{\rm ff})(t_n+\tau_m)+i(\Omega_n\tau_m+\phi_n^{(0)})}$$
$$\times \int_0^{t''} dt''' A_s(t'''-t_s-\tau_m) e^{i(\omega_{\rm fg}+V_{\rm ff}-\omega_s)(t'''-t_s-\tau_m)} e^{i(\omega_{\rm fg}+V_{\rm ff})(t_s+\tau_m)-i(\Omega_s\tau_m+\phi_s^{(0)})}, \quad \text{(S18)}$$

$$c^{(3,2)}_{\psi^+_{\rm ge}}(t) = \frac{i}{8}\sqrt{2}\mu_{\rm e}\mu_{\rm f}^2 \sum_{l,n,s=1}^{2} \int_0^t dt' A_l(t'-t_l-\tau_m) e^{-i(\omega_{\rm fg}-V_{\rm ee}-\omega_l)(t'-t_l-\tau_m)} e^{-i(\omega_{\rm fg}-V_{\rm ee})(t_l+\tau_m)+i(\Omega_l\tau_m+\phi_l^{(0)})}$$
$$\times \int_0^{t'} dt'' A_n(t''-t_n-\tau_m) e^{i(\omega_{\rm fg}-V_{\rm ee}-\omega_n)(t''-t_n-\tau_m)} e^{i(\omega_{\rm fg}-V_{\rm ee})(t_n+\tau_m)-i(\Omega_n\tau_m+\phi_n^{(0)})}$$
$$\times \int_0^{t''} dt''' A_s(t'''-t_s-\tau_m) e^{i(\omega_{\rm eg}+V_{\rm ee}-\omega_s)(t'''-t_s-\tau_m)} e^{i(\omega_{\rm eg}+V_{\rm ee})(t_s+\tau_m)-i(\Omega_s\tau_m+\phi_s^{(0)})}, \quad \text{(S19)}$$

$$c^{(3,\bar{2})}_{\psi^+_{\rm ge}}(t) = \frac{i}{8}\sqrt{2}\mu_{\rm e}\mu_{\rm f}^2 \sum_{l,n,s=1}^{2} \int_0^t dt' A_l(t'-t_l-\tau_m) e^{-i(\omega_{\rm fg}-V_{\rm ee}-\omega_l)(t'-t_l-\tau_m)} e^{-i(\omega_{\rm fg}-V_{\rm ee})(t_l+\tau_m)+i(\Omega_l\tau_m+\phi_l^{(0)})}$$
$$\times \int_0^{t'} dt'' A_n(t''-t_n-\tau_m) e^{i(\omega_{\rm eg}-V_{\rm ff}-\omega_n)(t''-t_n-\tau_m)} e^{i(\omega_{\rm eg}-V_{\rm ff})(t_n+\tau_m)-i(\Omega_n\tau_m+\phi_n^{(0)})}$$
$$\times \int_0^{t''} dt''' A_s(t'''-t_s-\tau_m) e^{i(\omega_{\rm fg}+V_{\rm ff}-\omega_s)(t'''-t_s-\tau_m)} e^{i(\omega_{\rm fg}+V_{\rm ff})(t_s+\tau_m)-i(\Omega_s\tau_m+\phi_s^{(0)})}, \quad \text{(S20)}$$

$$c^{(3,3)}_{\psi^+_{\rm ge}}(t) = \frac{i}{4}\sqrt{2}\mu_{\rm e}^3 \sum_{l,n,s=1}^{2} \int_0^t dt' A_l(t'-t_l-\tau_m) e^{-i(\omega_{\rm eg}-V_{\rm ee}-\omega_l)(t'-t_l-\tau_m)} e^{-i(\omega_{\rm eg}-V_{\rm ee})(t_l+\tau_m)+i(\Omega_l\tau_m+\phi_l^{(0)})}$$
$$\times \int_0^{t'} dt'' A_n(t''-t_n-\tau_m) e^{i(\omega_{\rm eg}-V_{\rm ee}-\omega_n)(t''-t_n-\tau_m)} e^{i(\omega_{\rm eg}-V_{\rm ee})(t_n+\tau_m)-i(\Omega_n\tau_m+\phi_n^{(0)})}$$
$$\times \int_0^{t''} dt''' A_s(t'''-t_s-\tau_m) e^{i(\omega_{\rm eg}+V_{\rm ee}-\omega_s)(t'''-t_s-\tau_m)} e^{i(\omega_{\rm eg}+V_{\rm ee})(t_s+\tau_m)-i(\Omega_s\tau_m+\phi_s^{(0)})}, \quad \text{(S21)}$$

$$c^{(1)}_{\psi^+_{\rm gf}}(t) = -\frac{i}{\sqrt{2}}\mu_{\rm f} \sum_{l=1}^{2} \int_{t_0}^t dt' A_j(t'-t_l-\tau_m) e^{i(\omega_{\rm fg}+V_{\rm ff}-\omega_j)(t'-t_j-\tau_m)} e^{i(\omega_{\rm fg}+V_{\rm ff})(t_j+\tau_m)-i(\Omega_j\tau_m+\phi_j^{(0)})}, \quad \text{(S22)}$$

$$c^{(3,1)}_{\psi^+_{\rm gf}}(t) \;=\; \frac{i}{4}\sqrt{2}\mu_{\rm f}^3 \sum_{l,n,s=1}^{2} \int_0^t dt' A_l(t'-t_l-\tau_m) e^{i(\omega_{\rm fg}+V_{\rm ff}-\omega_l)(t'-t_l-\tau_m)} e^{i(\omega_{\rm fg}+V_{\rm ff})(t_l+\tau_m)-i(\Omega_l\tau_m+\phi_l^{(0)})}$$
$$\times \int_0^{t'} dt'' A_n(t''-t_n-\tau_m) e^{-i(\omega_{\rm fg}+V_{\rm ff}-\omega_n)(t''-t_n-\tau_m)} e^{-i(\omega_{\rm fg}+V_{\rm ff})(t_n+\tau_m)+i(\Omega_n\tau_m+\phi_n^{(0)})}$$
$$\times \int_0^{t''} dt''' A_s(t'''-t_s-\tau_m) e^{i(\omega_{\rm fg}+V_{\rm ff}-\omega_s)(t'''-t_s-\tau_m)} e^{i(\omega_{\rm fg}+V_{\rm ff})(t_s+\tau_m)-i(\Omega_s\tau_m+\phi_s^{(0)})}, \quad \text{(S23)}$$

$$c^{(3,\bar{1})}_{\psi^+_{\rm gf}}(t) \;=\; \frac{i}{4}\sqrt{2}\mu_{\rm e}^2\mu_{\rm f} \sum_{l,n,s=1}^{2} \int_0^t dt' A_l(t'-t_l-\tau_m) e^{i(\omega_{\rm fg}+V_{\rm ff}-\omega_l)(t'-t_l-\tau_m)} e^{i(\omega_{\rm fg}+V_{\rm ff})(t_l+\tau_m)-i(\Omega_l\tau_m+\phi_l^{(0)})}$$
$$\times \int_0^{t'} dt'' A_n(t''-t_n-\tau_m) e^{-i(\omega_{\rm eg}+V_{\rm ee}-\omega_n)(t''-t_n-\tau_m)} e^{-i(\omega_{\rm eg}+V_{\rm ee})(t_n+\tau_m)+i(\Omega_n\tau_m+\phi_n^{(0)})}$$
$$\times \int_0^{t''} dt''' A_s(t'''-t_s-\tau_m) e^{i(\omega_{\rm eg}+V_{\rm ee}-\omega_s)(t'''-t_s-\tau_m)} e^{i(\omega_{\rm eg}+V_{\rm ee})(t_s+\tau_m)-i(\Omega_s\tau_m+\phi_s^{(0)})}, \quad \text{(S24)}$$

$$c^{(3,2)}_{\psi^+_{\rm gf}}(t) \;=\; \frac{i}{8}\sqrt{2}\mu_{\rm e}^2\mu_{\rm f} \sum_{l,n,s=1}^{2} \int_0^t dt' A_l(t'-t_l-\tau_m) e^{-i(\omega_{\rm eg}-V_{\rm ff}-\omega_l)(t'-t_l-\tau_m)} e^{-i(\omega_{\rm eg}-V_{\rm ff})(t_l+\tau_m)+i(\Omega_l\tau_m+\phi_l^{(0)})}$$
$$\times \int_0^{t'} dt'' A_n(t''-t_n-\tau_m) e^{i(\omega_{\rm eg}-V_{\rm ff}-\omega_l)(t''-t_n-\tau_m)} e^{i(\omega_{\rm eg}-V_{\rm ff})(t_n+\tau_m)-i(\Omega_n\tau_m+\phi_n^{(0)})}$$
$$\times \int_0^{t''} dt''' A_s(t'''-t_s-\tau_m) e^{i(\omega_{\rm fg}+V_{\rm ff}-\omega_l)(t'''-t_s-\tau_m)} e^{i(\omega_{\rm fg}+V_{\rm ff})(t_s+\tau_m)-i(\Omega_s\tau_m+\phi_s^{(0)})}, \quad \text{(S25)}$$

$$c^{(3,\bar{2})}_{\psi^+_{\rm gf}}(t) \;=\; \frac{i}{8}\sqrt{2}\mu_{\rm e}^2\mu_{\rm f} \sum_{l,n,s=1}^{2} \int_0^t dt' A_l(t'-t_l-\tau_m) e^{-i(\omega_{\rm eg}-V_{\rm ff}-\omega_l)(t'-t_l-\tau_m)} e^{-i(\omega_{\rm eg}-V_{\rm ff})(t_l+\tau_m)+i(\Omega_l\tau_m+\phi_l^{(0)})}$$
$$\times \int_0^{t'} dt'' A_n(t''-t_n-\tau_m) e^{i(\omega_{\rm fg}-V_{\rm ee}-\omega_n)(t''-t_n-\tau_m)} e^{i(\omega_{\rm fg}-V_{\rm ee})(t_n+\tau_m)-i(\Omega_n\tau_m+\phi_n^{(0)})}$$
$$\times \int_0^{t''} dt''' A_s(t'''-t_s-\tau_m) e^{i(\omega_{\rm eg}+V_{\rm ee}-\omega_n)(t'''-t_s-\tau_m)} e^{i(\omega_{\rm eg}+V_{\rm ee})(t_s+\tau_m)-i(\Omega_s\tau_m+\phi_s^{(0)})}, \quad \text{(S26)}$$

$$c^{(3,3)}_{\psi^+_{\rm gf}}(t) \;=\; \frac{i}{4}\sqrt{2}\mu_{\rm f}^3 \sum_{l,n,s=1}^{2} \int_0^t dt' A_l(t'-t_l-\tau_m) e^{-i(\omega_{\rm fg}-V_{\rm ff}-\omega_l)(t'-t_l-\tau_m)} e^{-i(\omega_{\rm fg}-V_{\rm ff})(t_l+\tau_m)+i(\Omega_l\tau_m+\phi_l^{(0)})}$$
$$\times \int_0^{t'} dt'' A_n(t''-t_n-\tau_m) e^{i(\omega_{\rm fg}-V_{\rm ff}-\omega_n)(t''-t_n-\tau_m)} e^{i(\omega_{\rm fg}-V_{\rm ff})(t_n+\tau_m)-i(\Omega_n\tau_m+\phi_n^{(0)})}$$
$$\times \int_0^{t''} dt''' A_s(t'''-t_s-\tau_m) e^{i(\omega_{\rm fg}+V_{\rm ff}-\omega_s)(t'''-t_s-\tau_m)} e^{i(\omega_{\rm fg}+V_{\rm ff})(t_s+\tau_m)-i(\Omega_s\tau_m+\phi_s^{(0)})}, \quad \text{(S27)}$$

$$c_{\psi_{\rm ee}}(t) \;=\; -\frac{1}{2}\mu_{\rm e}^2 \sum_{l,n=1}^{2} \int_{t_0}^t dt' A_l(t'-t_l-\tau_m) e^{i(\omega_{\rm eg}-V_{\rm ee}-\omega_l)(t'-t_l-\tau_m)} e^{i(\omega_{\rm eg}-V_{\rm ee})(t_l+\tau_m)-i(\Omega_l\tau_m+\phi_l^{(0)})}$$
$$\times \int_{t_0}^{t'} dt'' A_n(t''-t_n-\tau_m) e^{i(\omega_{\rm eg}+V_{\rm ee}-\omega_n)(t''-t_n-\tau_m)} e^{i(\omega_{\rm eg}+V_{\rm ee})(t_n+\tau_m)-i(\Omega_n\tau_m+\phi_n^{(0)})}, \quad \text{(S28)}$$

$$c_{\psi_{\rm ff}}(t) = -\frac{1}{2}\mu_{\rm f}^2 \sum_{l,n=1}^{2} \int_{t_0}^{t} dt' A_l(t'-t_l-\tau_m) e^{i(\omega_{\rm fg}-V_{\rm ff}-\omega_l)(t'-t_l-\tau_m)} e^{i(\omega_{\rm fg}-V_{\rm ff})(t_l+\tau_m)-i(\Omega_l\tau_m+\phi_l^{(0)})}$$
$$\times \int_{t_0}^{t'} dt'' A_n(t''-t_n-\tau_m) e^{i(\omega_{\rm fg}+V_{\rm ff}-\omega_n)(t''-t_n-\tau_m)} e^{i(\omega_{\rm fg}+V_{\rm ff})(t_n+\tau_m)-i(\Omega_n\tau_m+\phi_n^{(0)})}, \quad \text{(S29)}$$

$$c_{\psi_{\rm ef}^+}(t) = -\frac{1}{2\sqrt{2}}\mu_{\rm e}\mu_{\rm f} \sum_{l,m=1}^{2} \int_{t_0}^{t} dt' A_l(t'-t_l-\tau_m) e^{i(\omega_{\rm fg}-V_{\rm ee}-\omega_l)(t'-t_l-\tau_m)} e^{i(\omega_{\rm fg}-V_{\rm ee})(t_l+\tau_m)-i(\Omega_l\tau_m+\phi_l^{(0)})}$$
$$\times \int_{t_0}^{t'} dt'' A_n(t''-t_n-\tau_m) e^{i(\omega_{\rm eg}+V_{\rm ee}-\omega_n)(t''-t_n-\tau_m)} e^{i(\omega_{\rm eg}+V_{\rm ee})(t_n+\tau_m)-i(\Omega_n\tau_m+\phi_n^{(0)})}$$
$$-\frac{1}{2\sqrt{2}}\mu_{\rm e}\mu_{\rm f} \sum_{l,n=1}^{2} \int_{t_0}^{t} dt' A_l(t'-t_l-\tau_m) e^{i(\omega_{\rm eg}-V_{\rm ff}-\omega_l)(t'-t_l-\tau_m)} e^{i(\omega_{\rm eg}-V_{\rm ff})(t_l+\tau_m)-i(\Omega_l\tau_m+\phi_l^{(0)})}$$
$$\times \int_{t_0}^{t'} dt'' A_n(t''-t_n-\tau_m) e^{i(\omega_{\rm fg}+V_{\rm ff}-\omega_n)(t''-t_n-\tau_m)} e^{i(\omega_{\rm fg}+V_{\rm ff})(t_n+\tau_m)-i(\Omega_n\tau_m+\phi_n^{(0)})}. \quad \text{(S30)}$$

Note that the integrations above depend on the specific pulse shape. For a rectangular pulse, the time-ordered integrals can be exactly calculated and analytical solutions of (de)modulated signals are obtained as shown in the main text. For Gaussian pulses, it seems difficult to do the integrals analytically and then numerical integration is required. However, instead of time-ordered triple integrals involved in equations above, we find that only single and time-ordered double integrals (e.g. Eqs. (13) and (14) in the main text) are enough for the calculation of signals of collective excitations as demonstrated in the main text.
